# Supplementary material for: Execution Time Program Verification With Tight Bounds
Source: arXiv:2210.11105 source file (2022-10-20)
Supplement: Supplementary file 1 [file amortized.tex]

\chapter{Amortized Cost VCG algorithm}
\label{apend:amortized}

\begin{lstlisting}[language=ml,label=lis:wp-amortized,float=htb,caption={Weakest Precondition Implementation with Amortization - while case.}]
let rec wpc s phi verbose =
  match s with
    (...)
  | While (id, b, _) ->
      let inv, f, n, a, p = get_oracle id in
      let time_body = Mul (n, a) in
      ( AAnd (AAnd (inv, AGe (f, Cons 0)), AEq (p, Cons 0))
      , Sum (Mul (Sum (n, Cons 1), time_bexp b), time_body) )
\end{lstlisting}

\begin{lstlisting}[language=ml,label=lis:vc-amortized,float=htb,caption={VC Implementation with Amortization - while case.}]
let rec vc s phi : annot list =
  match s with
    (...)
  | While (id, b, s') ->
      let inv, f, n, a, p = get_oracle id in
      let b = annot_of_bexp b in
      let wp, t = wpc s' (AAnd(inv, AAnd (AGt (f, Var "k"), AEq (p, Var "pk")))) false in
      AImpl (AAnd (inv, b), ALe (f, n))
      :: AImpl (inv, AGe(p, Cons 0))
      :: AForall ( "k", AImpl ( AAnd (inv, AAnd (b, AEq (f, Var "k"))), wp) )
      :: AGe (Sub (Sum(a, p), Var "pk"), t)
      :: AImpl (AAnd (inv, ANeg b), phi)
      :: vc s' inv
\end{lstlisting}
