# Supplementary material for: Execution Time Program Verification With Tight Bounds
Source: arXiv:2210.11105 source file (2022-10-20)
Supplement: Supplementary file 2 [file exact.tex]

\chapter{Exact Cost VCG Algorithm}
\label{apend:exact}

\begin{lstlisting}[language=ml,label=lis:wp-exact,float=htb,caption={Weakest Precondition Implementation for Exact Costs.}]
let rec wpc s phi =
  match s with
    (...)
  | If (b, s1, s2) ->
      let wp1, _ = wpc s1 phi verbose in
      let wp2, t = wpc s2 phi verbose in
      let v_b = annot_of_bexp b in
      let tb = time_bexp b in
      (AAnd (AImpl (v_b, wp1), AImpl (ANeg v_b, wp2)), Sum (t, tb))
      (* TODO: fix max *)
  | For (id, i, a, b, s') ->
      let x = Lt (Var i, b) in
      let inv = get_oracle id in
      let _, tc = wpc s' inv verbose in
      ( inv, Sum (Mul (Sum (Sub (b, Cons a), Cons 2), time_bexp x), 
             Mul (Sum (Sub (b, Cons a), Cons 1), tc)))
\end{lstlisting}

\begin{lstlisting}[language=ml,label=lis:vc-exact,float=htb,caption={Verification Condition for \textit{for} loop.}]
let rec vc s phi : annot list =
  match s with
    (...)
  | For (id, _, a, b, s') ->
      let inv = get_oracle id in
      let x = ALt (Cons a, b) in
      AImpl (inv, x)
      :: AImpl (AAnd (inv, x), wp s' inv)
      :: AImpl (AAnd (inv, ANeg x), phi)
      :: vc s' inv
\end{lstlisting}
